# Supplementary material for: Grammatical Gender, Neo-Whorfianism, and Word Embeddings: A Data-Driven Approach to Linguistic Relativity
Source: arXiv:1910.09729 source file (2019-10-22)
Supplement: Supplementary file 1 [file appendix.pdf]

Confidential Review Copy. DO NOT DISTRIBUTE.

## A (Inanimate) NorthEuraLex Concepts

| Concept ID | English |
|---|---|
| Abend::N | evening |
| Abhang::N | slope |
| Abstand::N | gap |
| Ader::N | vein |
| Alter::N | age |
| Angelegenheit::N | matter |
| Anhöhe::N | elevation |
| Anzahl::N | count |
| Apfel::N | apple |
| Arbeit::N | work |
| Arm::N | arm |
| Art::N | sort |
| Arznei::N | medicine |
| Asche::N | ashes |
| Ast::N | limb |
| Atem::N | breath |
| Auge::N | eye |
| Bach::N | brook |
| Band::N | ribbon |
| Bart::N | beard |
| Bau::N | lair |
| Bauch::N | belly |
| Baum::N | tree |
| Beere::N | berry |
| Bein::N | leg |
| Berg::N | mountain |
| Besen::N | broom |
| Bett::N | bed |
| Beutel::N | pouch |
| Bild::N | picture |
| Birke::N | birch |
| Blatt::N | leaf |
| Blume::N | flower |
| Blut::N | blood |
| Boden::N | ground, soil |
| Bogen[Waffe]::N | bow |
| Boot::N | boat |
| Brei::N | mush |
| Brett::N | board |
| Brief::N | letter |
| Brot::N | bread |
| Brunnen::N | well |
| Brust::N | breast, chest |
| Brücke::N | bridge |

**Continued from previous column**

| Concept ID | English |
|---|---|
| Buch::N | book |
| Buchstabe::N | character |
| Bucht::N | cove |
| Busen::N | bosom |
| Butter::N | butter |
| Bündel::N | bundle |
| Dach::N | roof |
| Decke::N | blanket |
| Deckel::N | cover |
| Donner::N | thunder |
| Dorf::N | village |
| Dreck::N | filth |
| Ecke::N | corner |
| Ei::N | egg |
| Eimer::N | bucket |
| Eis::N | ice |
| Eisen::N | iron |
| Ellenbogen::N | elbow |
| Ende::N | end |
| Entfernung::N | distance |
| Erde::N | earth |
| Erzählung::N | story |
| Essen::N | meal |
| Faden::N | thread |
| Falle::N | trap |
| Farbe::N | paint |
| Feder::N | feather |
| Fehler::N | mistake |
| Fell::N | fur |
| Fenster::N | window |
| Ferse::N | heel |
| Festland::N | land |
| Fett::N | fat |
| Feuer::N | fire |
| Fieber::N | fever |
| Figur::N | figure |
| Finger::N | finger |
| Fingernagel::N | fingernail |
| Fleisch::N | meat |
| Fluss::N | river |
| Flügel::N | wing |
| Frost::N | frost |
| Funke::N | spark |
| Fuß::N | foot |
| Fußboden::N | floor |
| Gabel::N | fork |

Confidential Review Copy. DO NOT DISTRIBUTE.

**Continued from previous column**

| Concept ID | English |
|---|---|
| Gang::N | walk |
| Gast::N | guest |
| Gedanke::N | thought |
| Gedächtnis::N | memory |
| Gegend::N | area |
| Gegenstand::N | item |
| Gehirn::N | brain |
| Geist::N | spirit |
| Geld::N | money |
| Gelächter::N | laughter |
| Genick::N | nape |
| Geruch::N | odour |
| Geschenk::N | gift |
| Geschirr::N | dishes |
| Geschmack::N | flavour |
| Geschäft::N | business |
| Gesicht::N | face |
| Gespräch::N | talk |
| Gesundheit::N | health |
| Getreide::N | corn |
| Gewalt::N | violence |
| Gewehr::N | gun |
| Gewicht::N | weight |
| Gipfel::N | summit |
| Glas::N | glass |
| Glück::N | happiness |
| Gold::N | gold |
| Grab::N | grave |
| Gras::N | grass |
| Grenze::N | border |
| Griff::N | handle |
| Grube::N | pit |
| Grund::N | reason |
| Größe::N | size |
| Gürtel::N | belt |
| Haar::N | hair |
| Haken::N | hook |
| Hals::N | neck |
| Hand::N | hand |
| Handfläche::N | palm |
| Handtuch::N | towel |
| Haufen::N | heap |
| Haus::N | house |
| Haut::N | skin |
| Heim::N | home |
| Hemd::N | shirt |

**Continued from previous column**

| Concept ID | English |
|---|---|
| Herz::N | heart |
| Heu::N | hay |
| Hilfe::N | help |
| Himmel::N | sky |
| Hitze::N | heat |
| Holz::N | wood |
| Honig::N | honey |
| Horn::N | horn |
| Hose::N | trousers |
| Hunger::N | hunger |
| Hälfte::N | half |
| Höhe::N | height |
| Höhle::N | cave |
| Hügel::N | hill |
| Insel::N | island |
| Jahr::N | year |
| Kamm::N | comb |
| Kampf::N | fight |
| Kante::N | edge |
| Kehle::N | throat |
| Kessel::N | kettle |
| Kiefer[Anatomie]::N | jaw |
| Kiefer[Baum]::N | pine |
| Kinn::N | chin |
| Kirche::N | church |
| Kissen::N | pillow |
| Kiste::N | box |
| Klaue::N | claw |
| Kleidung::N | clothes |
| Knie::N | knee |
| Knochen::N | bone |
| Knopf::N | button |
| Knoten::N | knot |
| Kohle::N | coal |
| Kopf::N | head |
| Korn::N | grain |
| Kraft::N | force |
| Kragen::N | collar |
| Kralle::N | claw |
| Krankheit::N | illness |
| Kreis::N | circle |
| Kreuz::N | cross |
| Krieg::N | war |
| Kummer::N | grief |
| Kälte::N | chill |
| Körper::N | body |

Confidential Review Copy. DO NOT DISTRIBUTE.

**Continued from previous column**

| Concept ID | English |
|---|---|
| Küste::N | coast |
| Laden::N | shop |
| Lagerfeuer::N | campfire |
| Land::N | country |
| Last::N | load |
| Laut::N | sound |
| Leben::N | life |
| Leber::N | liver |
| Leder::N | leather |
| Lehm::N | clay |
| Leine::N | leash |
| Leiter::N | ladder |
| Leute::N | people |
| Licht::N | light |
| Lied::N | song |
| Linie::N | line |
| Lippe::N | lip |
| Loch::N | hole |
| Luft::N | air |
| Lust::N | desire |
| Länge::N | length |
| Lärm::N | noise |
| Löffel::N | spoon |
| Lüge::N | lie |
| Macht::N | power |
| Magen::N | stomach |
| Meer::N | sea |
| Menge::N | amount |
| Messer::N | knife |
| Milch::N | milk |
| Mittag::N | noon |
| Mitte::N | middle |
| Monat::N | month |
| Mond::N | moon |
| Moor::N | moor |
| Morgen::N | morning |
| Mund::N | mouth |
| Muster::N | pattern |
| Märchen::N | fairy tale |
| Mütze::N | cap |
| Nabel::N | navel |
| Nachricht::N | message |
| Nacht::N | night |
| Nadel::N | needle |
| Nagel::N | nail |
| Nagel[Anatomie]::N | nail |

**Continued from previous column**

| Concept ID | English |
|---|---|
| Nahrung::N | food |
| Name::N | name |
| Nase::N | nose |
| Nebel::N | fog |
| Nest::N | nest |
| Netz::N | net |
| Neuigkeit::N | news |
| Norden::N | north |
| Nutzen::N | profit |
| Oberschenkel::N | thigh |
| Ofen::N | stove |
| Ohr::N | ear |
| Ort::N | place |
| Osten::N | east |
| Pfad::N | path |
| Pfeil::N | arrow |
| Pilz::N | mushroom |
| Platte::N | slab |
| Platz::N | space |
| Preis::N | price |
| Puppe::N | doll |
| Quelle::N | source |
| Rand::N | fringe |
| Rauch::N | smoke |
| Raureif::N | hoarfrost |
| Rede::N | speech |
| Regal::N | shelf |
| Regen::N | rain |
| Regenbogen::N | rainbow |
| Reichtum::N | wealth |
| Reihe::N | row |
| Riemen::N | strap |
| Rinde::N | bark |
| Ring::N | ring |
| Rohr::N | pipe |
| Ruder::N | oar |
| Ruf::N | call |
| Ruhe::N | calm |
| Rätsel::N | puzzle |
| Rücken::N | back, spine |
| Saat::N | seed |
| Sache::N | thing |
| Sack::N | sack |
| Salz::N | salt |
| Sand::N | sand |
| Schaden::N | damage |

Confidential Review Copy. DO NOT DISTRIBUTE.

**Continued from previous column**

| Concept ID | English |
|---|---|
| Schale::N | husk |
| Schatten::N | shadow |
| Schaufel::N | shovel |
| Schaum::N | foam |
| Scheibe::N | slice |
| Schlaf::N | sleep |
| Schlinge::N | noose |
| Schlitten::N | sleigh |
| Schloss::N | lock |
| Schluss::N | conclusion |
| Schmerz::N | pain |
| Schmutz::N | dirt |
| Schnee::N | snow |
| Schnur::N | string |
| Schnurrbart::N | moustache |
| Schritt::N | step |
| Schuh::N | shoe |
| Schuld::N | fault |
| Schulter::N | shoulder |
| Schwanz::N | tail |
| See::N | lake |
| Sehne::N | sinew |
| Seite::N | side |
| Silber::N | silver |
| Sinn::N | meaning |
| Ski::N | ski |
| Sonne::N | sun |
| Spaten::N | spade |
| Speise::N | dish |
| Spiegel::N | mirror |
| Spiel::N | game |
| Spitze::N | tip |
| Sprache::N | language |
| Spur::N | track |
| Staat::N | state |
| Stab::N | staff |
| Stadt::N | town |
| Stamm::N | trunk |
| Stange::N | pole |
| Staub::N | dust |
| Stein::N | stone |
| Stern::N | star |
| Stiefel::N | boot |
| Stimme::N | voice |
| Stirn::N | forehead |
| Stock::N | stick |

**Continued from previous column**

| Concept ID | English |
|---|---|
| Stoff::N | cloth |
| Straße::N | road |
| Strich::N | stroke |
| Strömung::N | current |
| Stuhl::N | chair |
| Stärke::N | strength |
| Stück::N | piece |
| Stütze::N | bracket |
| Sumpf::N | swamp |
| Suppe::N | soup |
| Süden::N | south |
| Sünde::N | sin |
| Tag::N | day |
| Tanne::N | fir |
| Tasche::N | bag |
| Tasse::N | cup |
| Tee::N | tea |
| Teil::N | part |
| Tisch::N | table |
| Tod::N | death |
| Ton::N | tone |
| Topf::N | pot |
| Tor::N | gate |
| Traum::N | dream |
| Tropfen::N | drop |
| Träne::N | tear |
| Tuch::N | scarf |
| Tür::N | door |
| Ufer::N | shore |
| Unglück::N | misfortune |
| Verstand::N | mind |
| Volk::N | nation |
| Wahrheit::N | truth |
| Wald::N | forest |
| Wange::N | cheek |
| Ware::N | ware |
| Wasser::N | water |
| Weg::N | way |
| Weide::N | pasture |
| Weide[Baum]::N | willow |
| Welle::N | wave |
| Welt::N | world |
| Westen::N | west |
| Wetter::N | weather |
| Wiege::N | cradle |
| Wiese::N | meadow |

**Continued from previous column**

| Concept ID | English |
|---|---|
| Wind::N | wind |
| Winkel::N | angle |
| Woche::N | week |
| Wolke::N | cloud |
| Wolle::N | wool |
| Wort::N | word |
| Wunde::N | wound |
| Wunsch::N | wish |
| Wurzel::N | root |
| Zahn::N | tooth |
| Zaun::N | fence |
| Zeh::N | toe |
| Zeichen::N | sign |
| Zeit::N | time |
| Zeitung::N | newspaper |
| Zunge::N | tongue |
| Zweig::N | branch |
| Zwiebel::N | onion |
| Ärmel::N | sleeve |
| Öl::N | oil |
